# Supplementary material for: Stealthy Imitation: Reward-guided Environment-free Policy Stealing
Source: arXiv:2405.07004 source file (2024-05-11)
Supplement: Supplementary file 4 [file 07_rebuttal.tex]

\subsection{Rebuttal Objectives}

\begin{itemize}
    \item Increase score for Reviewers 3FCu and AqHM
    \item Keep / increase score for Reviewers LEDd and Maon
\end{itemize}

\subsection{Rebuttal Work Items}

\begin{enumerate}
    \item Clarify the scope of the paper (done)
    \item Include table showing the method difference and novelty (done)
    \item Include Diabetes results in rebuttal (done)
    \item Include Pandas experiments? (done)
    \item Perform new experiments if possible https://github.com/siemens/industrialbenchmark (Panda and Mujoco should be sufficient if Panda performs better)
    \item sensor but not the value
    \item Acknowledge the suggestions and update in pdf as list below
    \item reward model loss in appendix (done)
    \item change smoothl1's citation with huber loss paper, but keep the name (done)
    \item univariate to multivariate but with diagonal covariance matrix (done; we choose a multivariate normal distribution $\mathcal{N}(\vmu, \vsigma^2)$ with a diagonal covariance matrix as estimate of the attacker distribution) 
    \item KL figure start with 0 in y axis (done)
    \item dfme performance multiplying with large scale(NO,just reply in the rebuttal)
    \item check the reference number is correct for each reviewer
    \item panda appendix has additional page for single figure, is this ok?
    \item discuss where we are going to mention panda and reward model in main paper. (done; panda is in experimental setup, reward is in result)
    
    
\end{enumerate}

\subsection{Response to all reviewers}
\begin{markdown}

- **Why not consider higher dimensional RL scenario**: The considered scenario of this work is the industrial control system which does not use image as input. In this case, the dimension of mujoco includes high dimension task. If the input is image, we lose the motivation to estimate the input range as it should be in image format whose required range is already known as `[0,255]`. In contrary, industrial control systems that do not use image usually accepts different sensor values that have different semantics and ranges which the victim/target system does not want to disclose. We extend our method to a more realistic robot arm scenario describe in [1].

                                                         
- **Inspiration to image-based RL policy stealing**: While our current focus is not on image-based inputs, we acknowledge the potential complexity in such scenarios. Even with a known range for images, there likely exists specific "sub-ranges" within the embedding feature space that are crucial. We hope our current research inspires future investigations to identify these critical "sub-ranges" within image-based RL environments or even text-based. This approach would mark a shift from the current data-free model stealing methods, which predominantly focus on individual sample synthesizing, to a more nuanced exploration of embedding feature space.


\end{markdown}


\subsection{Response to Reviewer LEDd}
\begin{markdown}

We thank the reviewer for the thoughtful feedback. We are encouraged that the reviewer finds that policy stealing under the new threat model to be an advancement and that the countermeasure is practical. We aim to answer the reviewer's concerns in the following.


> Real-World Applicability: Transitioning from a controlled experimental setup to real-world applications might present unforeseen challenges


We add new experiments to validate Stealthy Imitation in realistic scenarios where the victim policies are trained for a Franka Emika Panda robot arm provided by panda-gym [1]. All victim policies are from official
repository in [HuggingFace](https://huggingface.co/sb3) and we focus on four out of five tasks, excluding the stacking task where the victim policy exhibited a 0\% success rate. In the four tasks we select, the maximum return is 0 and the minimum return is -50.

To demonstrate our method's efficacy, we initialize the estimated distribution with $\mathcal{N}(\mu^*+3\sigma^*,(\sigma^*)^2)$, thus all initial $D_{\mathrm{KL}}$ is 4.5, because initializing with $ \mathcal{N}(\mathbf{0}_n,\mathbf{1}_n^2)$ already results in a very small $D_{\mathrm{KL}}$ below 4.5. 

The table below summarizes task details and the percentage reduction in $D_{\mathrm{KL}}$ using Stealthy Imitation after 50M queries. We observe that Stealthy Imitation effectively reduces $D_{\mathrm{KL}}$ in most tasks, except Slide due to the lower victim return. Higher victim returns correlate with greater $D_{\mathrm{KL}}$ reductions. The attacker's return ratio reaches 100\% in the Reach task but is near 0\% in others, suggesting that precise distribution estimation is crucial for successful policy stealing in certain tasks.

| **Environment**         | **Observation space** | **Action space** | **Victim return** | **$D_{\mathrm{KL}}$ reduction** |
|-------------------------|-----------------------|------------------|-------------------|---------------------------------|
| PandaPickAndPlace-v1    | 26                    | 4                | -12±12            | 52%                             |
| PandaPush-v1            | 25                    | 3                | -6±2              | 59%                             |
| PandaReach-v1           | 13                    | 3                | -2±1              | 73%                             |
| PandaSlide-1            | 25                    | 3                | -29±13            | 4%                              |

We have updated the paper draft with complete experiments on the Panda tasks in Appendix G.

[1] Quentin Gallouédec, Nicolas Cazin, Emmanuel Dellandréa, and Liming Chen. panda-gym: Open-Source Goal-Conditioned Environments for Robotic Learning. Robot Learning Workshop: Self-Supervised and Lifelong Learning at NeurIPS, 2021

> Model stealing with a synthetic dataset + a surrogate model (here state estimators) is not new to the community.

We would like to emphasize that our method differs from standard model stealing by focusing on how to estimate the valid input range, while we do follow the standard way to steal policy after the estimation process. Additionally, if by "state estimators" here the reviewer refers to the estimated probability distribution, then it is also different from previous work which train a generator model through back-propagation. We also include a reward model which helps understand the imitation difficulty across regions. For a detailed explanation on how our method contrasts with DFME, please also see the answer to the next point.

> [...] the baseline of DFML is not fair enough given the different settings here.
> Following the philosophy of DFML, it seems that the proposed SI is the same approach under the RL setting.

Stealthy Imitation is the first method to steal a policy without the knowledge of input range, which means that there are no baselines for this setup. However, we want to provide a comparison to prior art and adapt DFME to the best of our ability to the present setup. 
We also summarize the difference between DFME and Stealthy Imitation in the following table; the two methods tackle different threat models and achieve different goals.  


| Method         | Data Source              | Target Feature            | Optimization Focus                            | Reusable                                                                     | Key Advantage                                                 |
|----------------|--------------------------|---------------------------|------------------------------------------------|---------------------------------------------------------------------------------|---------------------------------------------------------------|
| DFME    | Model-generated data     | Adversarial examples      | Sample difficulty with $L_1$ loss | Not, as adversarial examples vary from model to model              | Refines data distribution using knowledge of input range |
| Ours   | Probability distribution | Hard-to-Imitate Region   | Overall difficulty with reward model | Yes, as the input range does not change           | Efficiently estimates input range                 |

> challenges of this matter, especially the unique challenges when applying such attack in the RL setting

The main challenge is the potentially unbounded input space and the valid range being unknown to the attacker. Current model stealing mainly focuses on the image domain, where the input range is known (i.e., pixel range [0,255]). This premise does not hold in, e.g., industrial control systems, where variables have varying semantics and scales (e.g., sensor data). For these systems, the model is often trained using RL instead of supervised learning.
We show that such RL models can also be stolen using supervised learning on synthetic data (Sec. 5.3, Distribution approximation), as long as the attacker knows the input distribution.
In this setup, the difficulty thus becomes the input distribution estimation, which we solve as part of our contribution.

\end{markdown}


\subsection{Response to Reviewer 3FCu}


\begin{markdown}

We thank the reviewer for the insightful and positive feedback. We are pleased to see that the reviewer found the idea and challenges new and potentially applicable across different domains. We answer their questions below.

> The test environments are quite limited. These Mujoco environments are small, and there are only three of them.

To answer the reviewer's concern, we include new experiments to validate Stealthy Imitation in realistic scenarios where the victim policies are trained for a Franka Emika Panda robot arm provided by panda-gym [1]. All victim policies are from official
repository in [HuggingFace](https://huggingface.co/sb3) and we focus on four out of five tasks, excluding the stacking task where the victim policy exhibited a 0\% success rate. In the four tasks we select, the maximum return is 0 and the minimum return is -50.

To demonstrate our method's efficacy, we initialize the estimated distribution with $\mathcal{N}(\mu^*+3\sigma^*,(\sigma^*)^2)$, thus all initial $D_{\mathrm{KL}}$ is 4.5, because initializing with $ \mathcal{N}(\mathbf{0},\mathbf{1})$ already results in a very small $D_{\mathrm{KL}}$ below 4.5. 

The table below summarizes task details and the percentage reduction in $D_{\mathrm{KL}}$ using Stealthy Imitation after 50M queries. We observe that Stealthy Imitation effectively reduces $D_{\mathrm{KL}}$ in most tasks, except Slide due to the lower victim return. Higher victim returns correlate with greater $D_{\mathrm{KL}}$ reductions. The attacker's return ratio reaches 100\% in the Reach task but is near 0\% in others, suggesting that precise distribution estimation is crucial for successful policy stealing in certain tasks.

| **Environment**         | **Observation space** | **Action space** | **Victim return** | **$D_{\mathrm{KL}}$ reduction** |
|-------------------------|-----------------------|------------------|-------------------|---------------------------------|
| PandaPickAndPlace-v1    | 26                    | 4                | -12±12            | 52%                             |
| PandaPush-v1            | 25                    | 3                | -6±2              | 59%                             |
| PandaReach-v1           | 13                    | 3                | -2±1              | 73%                             |
| PandaSlide-1            | 25                    | 3                | -29±13            | 4%                              |

We have updated the paper draft with complete experiments on the Panda tasks in Appendix G.

[1] Quentin Gallouédec, Nicolas Cazin, Emmanuel Dellandréa, and Liming Chen. panda-gym: Open-Source Goal-Conditioned Environments for Robotic Learning. Robot Learning Workshop: Self-Supervised and Lifelong Learning at NeurIPS, 2021

> This method seems impossible for policies with high-dimensional input such as images.

We want to clarify that image data does not fit the setup of the knowledge-limited attacker we consider.
Particularly, the input range is known for the image domain (i.e., pixel values in [0,255]). For this case, classic existing model stealing methods can be applied.


> The approximation of the state distribution using a normal distribution seems quite limiting

We argue that the capacity to estimate states based on a normal distribution is a feature of our method.
We show that this assumption is sufficient to approximate more complex distributions; this finding is part of the paper's contributions.
The experimental results on the Panda robot arm show that this assumption holds for high dimensional state spaces (26 dimensions for the Panda Pick And Place task).


> circumvent defense by querying multiple times

We agree with the reviewer that tackling security topics often involves a cat and mouse game between the attacker and the defender.
Building on the reviewer's attack suggestion, our defense can be enhanced to produce responses with similar variance for queries outside the range as those within range. For instance, the defender could map queries outside the range to a random or fixed point within the range, resulting in a similar output variance. We appreciate this discussion and will incorporate it into the revised draft of our paper.

> [...] it will get better at the regions of space most recently encountered, and may lose capability on regions that have not been visited recently.

We believe the reviewer's understanding is correct. We clarify that the distribution shift across iterations is indeed intentional and a key part of our method in search of the correct victim distribution. The evaluator $\pi_e$ plays a crucial role in selecting the most suitable distribution. The final attacker policy only needs to perform well on the distribution chosen by $\pi_e$, not on all explored distributions.


> The authors target interactive policies in RL domains, but there doesn't seem to be anything here requiring RL, or specific to the RL setting.

We thank the reviewer for highlighting the general potential of our method. We include here results for Stealthy Imitation applied to binary classification on the Diabetes dataset [1]. The input consists of eight variables and has different semantics and scales; the output can be considered as a continuous "action" between [0,1]. We initialize the estimated distribution with $\mathcal{N}(\mu^+3\sigma^,(\sigma^*)^2)$, instead of $ \mathcal{N}(\mathbf{0}_n,\mathbf{1}_n^2)$ which results in high $D_{\mathrm{KL}}$ (2712). The accuracy of the victim model is 77\%. The final attacker model can achieve 69\% accuracy (90\% w.r.t. the victim) and the $D_{\mathrm{KL}}$ also has a decreasing trend as shown below.

| Iteration         | 0   | 2   | 4   | 6   | 8   | 10  | 12  |
|-------------------|-----|-----|-----|-----|-----|-----|-----|
| $D_{\mathrm{KL}}$ | 4.5 | 4.4 | 4.0 | 3.6 | 3.2 | 3.1 | 3.1 |

While we acknowledge the potential of Stealthy Imitation beyond RL contexts (e.g., feature vectors, multivariate time series), we leave the in-depth analysis of these applications to future work.

[1] Kahn, Michael. Diabetes. UCI Machine Learning Repository. https://doi.org/10.24432/C5T59G.

\end{markdown}

\subsection{Response to Reviewer AqHM}
\begin{markdown}

We thank the reviewer for their constructive comments and valuable suggestions. It is encouraging that the reviewer finds the paper novel and comprehensive. We answer their questions as follows.

> 1. There are some additional issues with some of the exposition being unclear or misleading:[...]

We appreciate the suggestions for improving the clarity of the paper and have incorporated them into our revised draft.

> 2. Why is the objective in (1) to minimize reward difference? Shouldn't it either be to maximize reward, or imitate as precisely as possible?

Minimizing reward difference focuses on the target of replicating the functionality of the victim policy, as opposed to obtaining the best possible performance on the task. This goal of functional stealing is standard throughout model stealing literature [1].
Additionally, it is common in inverse RL [2] to learn a reward function that measures the actions in the context of the overall goal, rather than scoring the replicating of individual actions. For instance, consider the following pathological case: if an attacker policy imitates only the second half of a victim policy's actions in a sequence, the action agreement is 50\%. However, differing actions in the first half could result in zero returns for the attacker policy due to cascading effects, highlighting the significance of targeting the end goal, rather than exact action replication.


> 3. What is the point of stealing a policy if you don't know the environment?

We consider two reasons why an attacker might seek to steal a policy without knowledge of the environment:

Firstly, **further attacks**: stealing a policy enables the attacker to disrupt the target control system. They can generate adversarial signals with the stolen policy, even without understanding the environment.

Secondly, **sensitive information exposure and unauthorized usage**: it enables the attacker to access confidential information, like sensor types or preprocessing methods. The information could potentially aid in the development of their own control system.


> 4. What exactly is the purpose of the experiments in Figure 3, since to calculate all of these distributions one needs access to states sampled from $\mathbb{S}_v$, which is not possible under the threat model proposed? Why not compare to $\mathcal{N}(\tilde{\mu},\tilde{\sigma}^2)$ as well?

This experiment is conducted from an analytical viewpoint, rather than that of an attacker. This goes for the entire analysis and ablations section (Sec. 5.3). This experiment in particular explores the minimal knowledge required for successful policy stealing. It highlights the risk associated with exposing input distributions, even through a normal distribution, and demonstrates that RL-trained policies in control systems can be compromised using supervised learning. Since the attacker cannot access $\mathbb{S}_v$, Stealthy Imitation does not utilize it. The outcomes using the attacker's approximation, $\mathcal{N}(\tilde{\mu},\tilde{\sigma}^2)$, are displayed at the bottom of Figure 2, marked as "ours".


> 5. What exactly is the initial state range output by DFME, and what happens if you expand the initial range? For instance, one could simply use a larger weight initialization for the final layer of the generator network in DFME, or multiply the outputs by a large constant. How does this compare to the newly proposed SI attack?

We aligned DFME's initial state output distribution with ours $ \mathcal{N}(\mathbf{0}_n,\mathbf{1}_n^2)$. The original DFME generator used a tanh activation function, confining outputs to [-1,1], typical in image classification model stealing. We adapt DFME to the best of our ability to the present setup by substituting this with `**batch normalization with learnable scaling and shift factors**`, enabling the generator to explore regions beyond the $ \mathcal{N}(\mathbf{0}_n,\mathbf{1}_n^2)$ starting point.

Additionally, we follow the reviewer's suggestion and amplify the output of the DFME generator by factors of 10 and 100. The resulting return ratio of the attacker policy in these two additional experiments is worse than before throughout 50M queries.


[1] Tribhuvanesh Orekondy, Bernt Schiele, and Mario Fritz. Knockoff nets: Stealing functionality of black-box models. In Conference on Computer Vision and Pattern Recognition (CVPR), pp. 4954–4963, 2019b.

[2] Ng, Andrew Y., and Stuart Russell. Algorithms for inverse reinforcement learning. ICML. 2000.

\zzx{In contrast, our approach involves training a reward model that provides a global perspective, identifying regions that are more challenging to mimic. This allows us to directly adjust the probability distribution, rather than concentrating on single data points.}

\end{markdown}

\subsection{Response to Reviewer Maon}

\begin{markdown}

We appreciate the thoughtful and beneficial feedback provided by the reviewer. We are pleased that reviewer find the challenges beyond supervised model stealing clear. We would like to address the following questions:

> While the threat model is realistic, the application seems simple.

We add new experiments to validate Stealthy Imitation in realistic scenarios where the victim policies are trained for a Franka Emika Panda robot arm provided by panda-gym [1]. Please see our [general comment about Validation of Applicability in Realistic Scenarios](https://openreview.net/forum?id=7q7s5fXEpP&noteId=ebtZUbFh9r) for a summary. We have also updated the paper draft to include the experiment details on the Panda tasks, which you can find in Appendix G


> This is particularly important given that model stealing is particularly relevant with large models only available as API such as the recent RT-2-X model [1]. 

We want to clarify that image models such as RT-2-X do not fit the setup of the knowledge-limited attacker we consider.
Particularly, the input range is known for the image domain (i.e., pixel values in [0,255]). For this case, classic existing model stealing methods can be applied.


> The performance of the victim policy+defense is not shown.

The performance of the victim policy with defense in a normal operating environment remains unchanged compared to without defense. This is because the defender only outputs incorrect actions when the queried state falls outside the valid input range. 

> The performance of the learned reward discriminator is not shown.

The loss of the reward discriminator exhibits oscillations with the variation of the estimated distribution and attacker policy through the iterations (similar to GAN pipelines).
We have updated the paper draft with the reward discriminator's loss in Appendix F.

> What would the required budget be to scale to image or lidar inputs?

As clarified previously, the assumptions of an unknown input range to the attacker does not hold for images or lidar. As such, this extension is not within the scope of the paper.

> Is there perhaps a way to break the defense along the lines of adaptive attacks proposed in (Tramer et al. "On Adaptive Attacks to Adversarial Example Defenses." 2020.)?

We would like to emphasize that [Tramer et al., 2020] and other results in that line of work address adversarial examples, a different type of security threat than model stealing; as such, these are not directly applicable to our setup.

Nevertheless, we can consider the consequences of the attacker becoming aware of the defense strategy.
In that case, our defense can be enhanced to produce responses with similar variance for queries outside the range as those within range.
For more details, please also see our answer to Reviewer 3FCu on possible attack variations.
Could the reviewer let us know if these variations answer the scenarios they had in mind?

[1] Quentin Gallouédec, Nicolas Cazin, Emmanuel Dellandréa, and Liming Chen. panda-gym: Open-Source Goal-Conditioned Environments for Robotic Learning. Robot Learning Workshop: Self-Supervised and Lifelong Learning at NeurIPS, 2021

\end{markdown}
