# Supplementary material for: Stealthy Imitation: Reward-guided Environment-free Policy Stealing
Source: arXiv:2405.07004 source file (2024-05-11)
Supplement: Supplementary file 5 [file 16_icml_rebuttal.tex]

I move the rebuttal into a collaborative platform, which supports real time compiling. Better than Overleaf. check the link below:

https://hackmd.io/@iX3zoOdwQFym_C5VBKcwOQ/HJuNuW0Ra/edit
